# Supplementary material for: Phonon transport unveils the prevalent point defects in GaN
Source: arXiv:1712.08124 source file (2017-12-21)
Supplement: Supplementary file 1 [file Supplementary.pdf]

# Phonon transport unveils the prevalent point defects in GaN: Supplementary Material

Ankita Katre[1],* Jesús Carrete[2], Tao Wang[3], Georg K. H. Madsen[2], and Natalio Mingo[1]†
[1] *LITEN, CEA-Grenoble, 17 rue des Martyrs, 38054 Grenoble Cedex 9, France*
[2] *Institut für Materialchemie, Technische Universität Wien, a-1060 Vienna, Austria and*
[3] *AMS, ICAMS, Ruhr-Universität Bochum, 44801 Bochum, Germany*

* ankitamkatre@gmail.com
† natalio.mingo@cea.fr

## I. COMPUTATIONAL DETAILS

The structural parameters for wurtzite-GaN (spacegroup $P6_3mc$) and the atomic forces required to determine interatomic force constants (IFCs) are calculated from first principles. The projector-augmented-wave method [1] implemented in the density functional theory package VASP [2] with the local density approximation for exchange and correlation [3] is used for these calculations. The lattice parameters for the obtained relaxed structure of GaN are $a = 3.15$ Å, $c = 5.14$ Å and the wurtzite parameter is $u = 0.38$ Å.

Next, the harmonic ($2^{\mathrm{nd}}$ order) and anharmonic ($3^{\mathrm{rd}}$ order) IFCs are computed within finite displacement appraoch for a supercell of $4 \times 4 \times 2$ of the hexagonal primitive cell, containing 128 atoms. To check the convergence, the harmonic IFCs are also obtained for a $5 \times 5 \times 3$ supercell and the maximum difference of 0.4 rad/ps is found for the angular frequencies $\omega$ at the $\Gamma$-point.

The harmonic IFCs for native and substitutional defects $\mathrm{Mg_{Ga}}$, $\mathrm{O_N}$, $V_{\mathrm{Ga}}$ and $V_{\mathrm{N}}$ are calculated for $4 \times 4 \times 2$ with one defect atom. The IFCs corresponding to the coupled defects $\mathrm{Mg_{Ga}}$-$\mathrm{O_N}$, $\mathrm{Mg_{Ga}}$-$V_{\mathrm{N}}$, $V_{\mathrm{Ga}}$-$\mathrm{O_N}$ and clustered defect $V_{\mathrm{Ga}}$-$(\mathrm{O_N})_3$ are also calculated in $4 \times 4 \times 2$ supercells with respectively two and four defect atoms.

The calculations are performed for energetically favourable charged states for these defects and both long and short orientations of the coupled and clustered defects are considered. Several iterations of the relaxation of the atomic coordinates (fixed cell volume) in the defective supercells are performed. This is done to avoid any imaginary phonon frequencies at the $\Gamma$-point of the Brillouin zone for the supercell.

The harmonic and anharmonic IFCs are extracted from calculated *ab-initio* forces using Phonopy [4] package and our own thirdorder.py code [5] respectively.

We also include the Born effective charges and the dielectric tensor to account for non-analytical correction to the dynamical matrix and reproduce LO-TO (Longitudinal Optic and Transverse Optic) phonon splitting in GaN [6]. These are calculated using VASP.

The defect scattering rates are calculated on a uniformly spaced **q**-point mesh of $26 \times 26 \times 14$ with a $18 \times 18 \times 10$ grid for the Green's functions using the tetrahedron method to integrate over the Brillouin-zone [7]. Using a sparser grid for the Green's function than for the Brillouin zone integrations can mean that the elastic component of the scattering rates is not well reproduced at very low frequencies. However, in this region the precise value of that component is not relevant for the value of $\kappa$, since three-phonon scattering dominates. Using a coarser grid is thus innocuous, and very interesting for saving computational time. Green's functions, the scattering rates $\tau_{\mathrm{anh}}^{-1}$, $\tau_{\mathrm{iso}}^{-1}$ and $\tau_{\mathrm{def}}^{-1}$ and the final $\kappa$ are computed using our almaBTE code [8].

## II. GaN THERMAL CONDUCTIVITY WITH DIFFERENT DEFECTS

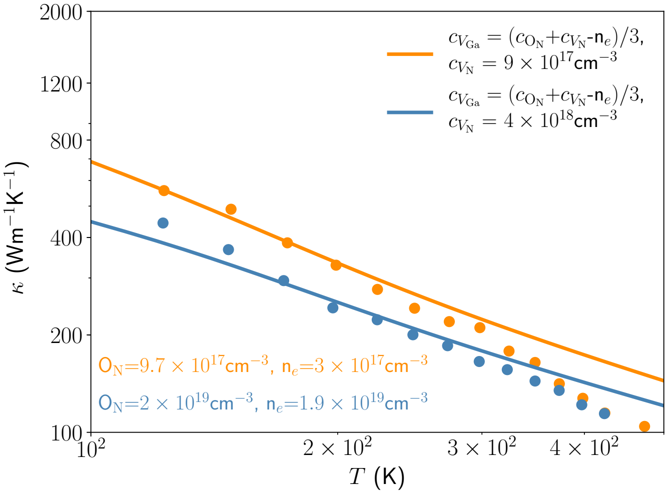


FIG. 1: GaN $\kappa$ calculated considering additional donor impurity $V_{\mathrm{N}}$ and compensating $V_{\mathrm{Ga}}$ in O-doped GaN samples [9]. $\kappa$ is reproduced by adjusting the vacancy concentrations and conserving the free carrier concentrations ($\mathrm{n}_e$) and the $c_{\mathrm{O_N}}$ as reported in ref. 9. The calculated thermal conductivity has a different slope than the experiments. Furthermore, the $V_{\mathrm{N}}$ concentrations which had to be used to get quantitative agreements with the experiments are very high and energetically unfavourable as discussed in the main text.

| | $O_N$ ($cm^{-3}$) | $n_e$ ($cm^{-3}$) | $V_{Ga}$ ($cm^{-3}$) | $V_N$ ($cm^{-3}$) | $\kappa_{calc}$ ($Wm^{-1}K^{-1}$) | $\kappa_{exp}$ ($Wm^{-1}K^{-1}$) |
|---|---|---|---|---|---|---|
| Experimental Sample-1 from ref. 9 | | | | | | |
| Test-1 | $0.97\times10^{18}$ | $0.3\times10^{18}$ | $0.22\times10^{18}$ | - | 239 | 211 |
| Test-2 | $0.97\times10^{18}$ | $0.3\times10^{18}$ | $0.52\times10^{18}$ | $0.9\times10^{18}$ | 223 | 211 |
| Experimental Sample-2 from ref. 9 | | | | | | |
| Test-1 | $20\times10^{18}$ | $19\times10^{18}$ | $0.32\times10^{18}$ | - | 221 | 166 |
| Test-2 | $20\times10^{18}$ | $19\times10^{18}$ | $1.67\times10^{18}$ | $4\times10^{18}$ | 179 | 166 |

TABLE I: Calculated thermal conductivity ($\kappa_{calc}$) at 300 K for different defect contents in O-doped GaN and compared to the experiments ($\kappa_{exp}$) from ref. 9. These tests, as explained in the main text, correspond to gallium vacancy concentrations: $c_{V_{Ga}}=\frac{1}{3}(c_{O_N}-n_e)$ and $c_{V_{Ga}}=\frac{1}{3}(c_{O_N}+c_{V_N}-n_e)$ respectively.

## III. PHONON-DEFECT SCATTERING RATES FOR DIFFERENT ORIENTATIONS OF COUPLED DEFECTS IN GaN.

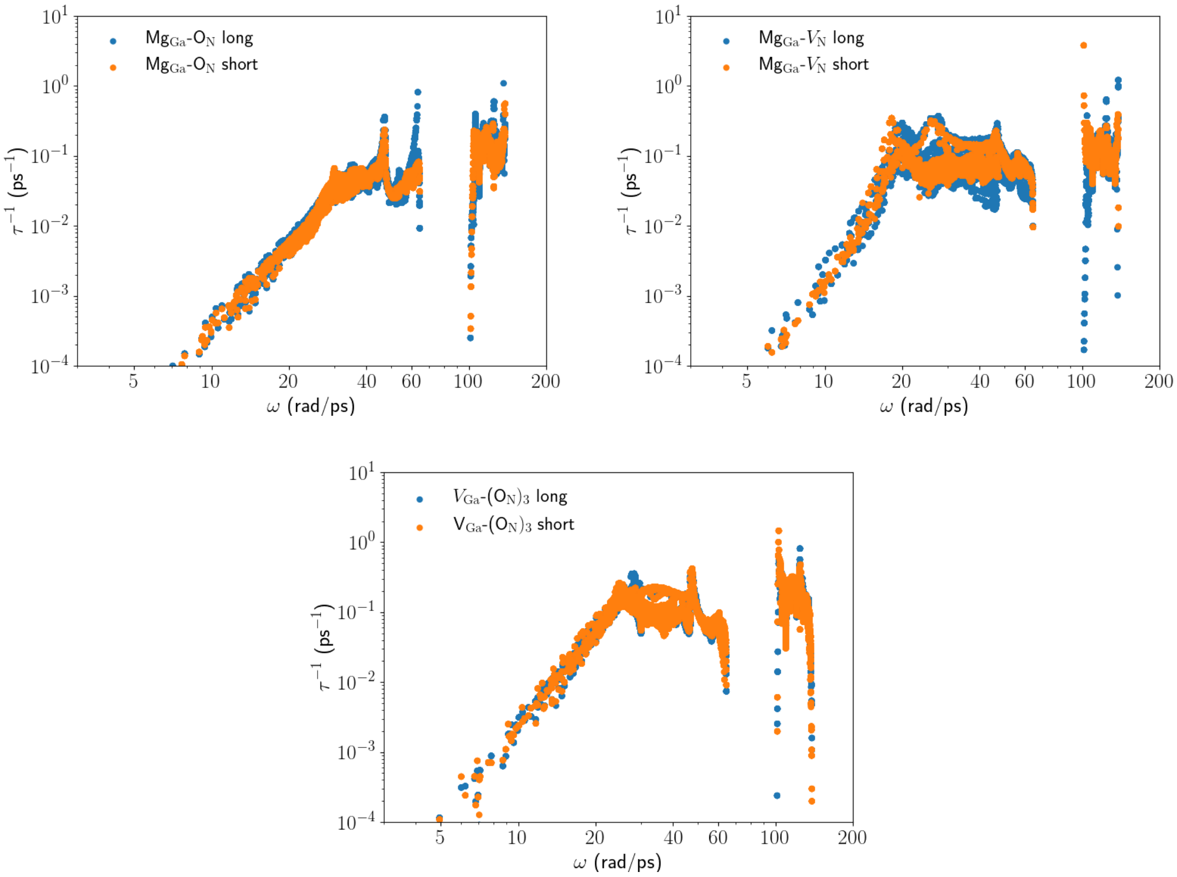


FIG. 2: Phonon-defect scattering rates ($\tau^{-1}$) calculated for long (with larger Ga-N bondlength) and short (with smaller Ga-N bondlength) orientations of (a) $Mg_{Ga}$-$O_N$ (b) $Mg_{Ga}$-$V_N$ and (c) $V_{Ga}$-$(O_N)_3$ clustered defect. Similar scattering rates are found for different orientations for these defects.

## IV. COMPARISON OF SCATTERING RATES FOR COUPLED AND SINGLE DEFECTS

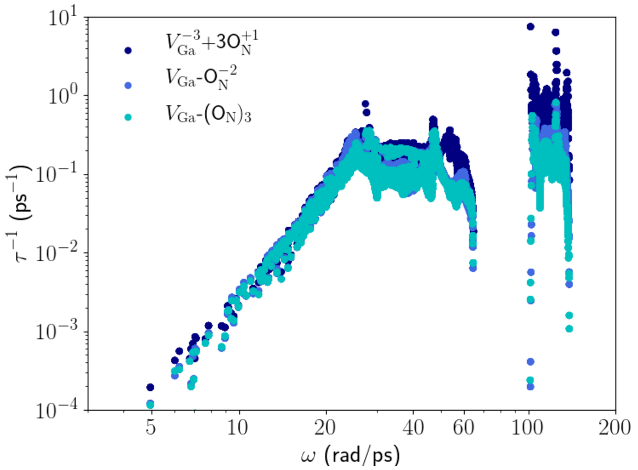


FIG. 3: Phonon-defect scattering rates for the cases of coupled and clustered vacancy-oxygen defects compared to the sum of scattering rates from individual isolated vacancy and oxygen defects. The similar results obtained for all three cases show that phonon scattering is unaffected by whether or not oxygens couple with gallium vacancies.

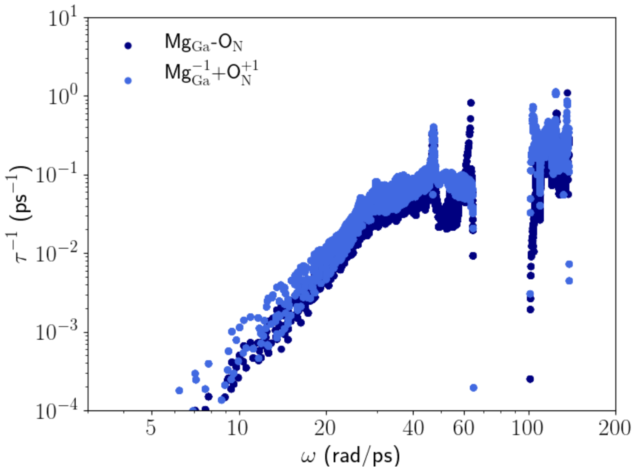


FIG. 4: Coupled magnesium-oxygen defect scattering rates compared to the sum of individual magnesium and oxygen defect scattering rates.

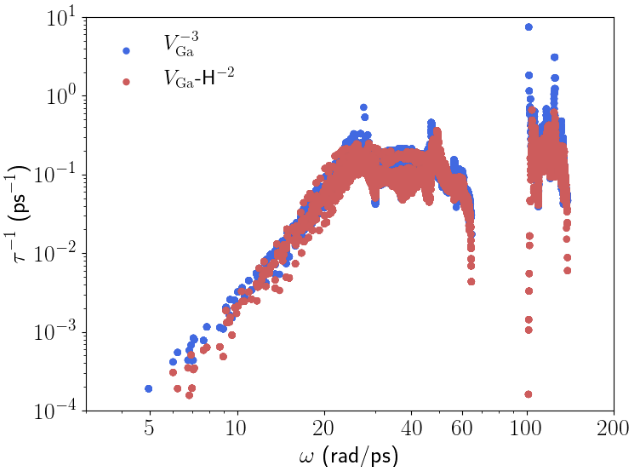


FIG. 5: Phonon-defect scattering rates for coupled vacancy-hydrogen defect compared with isolated vacancy. Hydrogens relax closer to nitrogens surrounding vacancies and dominant effect of only vacancy is seen on the phonon scattering.

[1] P. E. Blöchl, Physical Review B **50**, 17953 (1994).
[2] G. Kresse and D. Joubert, Physical Review B **59**, 1758 (1999).
[3] J. P. Perdew and A. Zunger, Physical Review B **23**, 5048 (1981).
[4] A. Togo, F. Oba, and I. Tanaka, Physical Review B **78**, 134106 (2008).
[5] W. Li, J. Carrete, N. A. Katcho, and N. Mingo, Computer Physics Communications **185**, 1747 (2014).
[6] Y. Wang, J. J. Wang, W. Y. Wang, Z. G. Mei, S. L. Shang, L. Q. Chen, and Z. K. Liu, Journal of Physics: Condensed Matter **22**, 202201 (2010).
[7] P. Lambin and J. P. Vigneron, Physical Review B **29**, 3430 (1984).
[8] J. Carrete, B. Vermeersch, A. Katre, A. Roekeghem, T. Wang, G. K. H. Madsen, and N. Mingo, Computer Physics Communications **220**, 351 (2017).
[9] R. B. Simon, J. Anaya, and M. Kuball, Applied Physics Letters **105**, 202105 (2014).
